# Supplementary material for: Closed-form congestion control via deep symbolic regression
Source: arXiv:2405.01435 source file (2024-03-28)
Supplement: Supplementary file 1 [file appendix.tex]

\appendix
\section{TD3 parameters}
\begin{lstlisting}[language=Python, caption=RLlib's TD3 parameters.]
"twin_q": True,
"policy_delay": 2,
"smooth_target_policy": True,
"target_noise": 0.05,
"target_noise_clip": 0.1,

"exploration_config": {
    "type": "GaussianNoise",
    "random_timesteps": 100000,
    "stddev": 0.1,
    "initial_scale": 1.0,
    "final_scale": 1.0,
    "scale_timesteps": 1e7,
},

"actor_hiddens":  [512, 16, 512],
"critic_hiddens": [512, 16, 512],

"n_step": 5,
"gamma": 0.999,
"actor_lr": 1e-5,
"critic_lr": 5e-5,
"l2_reg": 0,
"tau": 5e-5,
"target_network_update_freq": 0,
"rollout_fragment_length": 5,
"sample_async": True,

"buffer_size": 2000000,
"prioritized_replay": True,
"prioritized_replay_alpha": 0.2,
"prioritized_replay_beta": 0.2,
"prioritized_replay_beta_annealing_timesteps": 2e7,
"final_prioritized_replay_beta": 1.0,
"prioritized_replay_eps": 1e-6,
"compress_observations": False,
\end{lstlisting}
